# Supplementary material for: Programming Scalable Cloud Services with AEON
Source: arXiv:1912.03506 source file (2019-12-07)
Supplement: Supplementary file 1 [file appendix-language.tex]

\section{Proofs}
\label{sec:proofs}
% \gp{Expletive!!!, all the $(\acontextset, \aeventset)$ pairs are
%   reversed. You will learn to use macros x100. I think it's fixed
%   now.}

In this appendix we provide the full proofs for the claims made
in~\autoref{sec:semantics}. 
Let us first present some basic remarks about the semantic rules
of~\aeoncore{} presented in~\autoref{sec:semantics}. 

\begin{remark}
  \label{rem:commit}
  If an event $\aeid$ is executing within a context $\acontext[]$, 
  then $\aeid \in \acontext[].A$. That is, only activated
  events can execute within a context.
\end{remark}
\begin{proof}
  It suffices to see that the \textsc{Lift Intra} rule requires the
  event to be in the activation set to execute. All the other global
  rules do not execute within the context (i.e. do not make use of the
  $\hookrightarrow$ transitions of~\autoref{fig:big-step}). Similarly,
  activation rules do not ``execute'' within the context -- that is,
  they don't modify any of the components of the context other than the
  activation sets.
\end{proof}

\begin{remark}
  \label{rem:return-commit}
  The only rule that allows removing an event from activations is
  \textsc{Event Return \& Commit}, which completely removes the event
  from the configuration set.
\end{remark}
\proof{Simple observation of the semantic rules.}

\begin{corollary}
  \label{lem:lock-no-unlock}
  Consider a configuration $(\aeventset, \acontextset)$, an event
  $\aeid \in \aeventset$, and a context $\acontext[0]$ such that
  $\aeid \in \activated{\acontext[0]}$. Moreover, assume that
  $(\aeventset, \acontextset \cup \{\acontext[0]\}) \xrightarrow{*}
  (\aeventset', \acontextset' \cup \{\acontext[0]'\})$
  where $\aeid \in \aeventset'$.  Then we have that
  $\aeid \in \activated{\acontext[0]'}$. In other words, once an event
  is activated in a context, it remains so, until completely
  eliminated from the event set $\aeventset'$.
\end{corollary}
\begin{proof}
  This property is a simple consequence of~\autoref{rem:commit}. Since
  the only rule that can de-activate an event from a contexts
  eliminates the event from the activations of all contexts at once.
\end{proof}

\begin{remark}
  For any reachable configuration $\aconf$ such that a context
  $\acontext$ occurs in $\acontextset$ we have that either $|\acontext.A|
  \leq 1$, or every activation in is $\readonly$.
\end{remark}
\begin{proof}
  This is immediate from the antecedents of the activation rules
  (\autoref{fig:activation}). In particular, notice that
  \textsc{Exclusive} access rules require that the initial activation
  set be empty, and \textsc{ReadOnly} rules require that no exclusive
  access event is in the current activation set
  ($\exclusive \notin \acontext.A$).
\end{proof}

\paragraph{Deadlock Freedom.}~Let us refresh the definition of deadlock provided
in~\autoref{def:deadlock}. 

\begin{definition}[Deadlock State]
  We say a state $(\aeventset, \acontextset)$ contains a
  deadlock, if $\acontextset$ can be decomposed as:\\[2pt]
  \centerline{
    \( \acontextset = \acontextset' \cup \{\acontext[0], \acontext[1], \dots,
    \acontext[n]\} \)
  }\\[2pt]
  where for each $i \in [0,n]$ we have that there exists an event
  $\aeid[i] \in \aeventset$ such that: (i)
  $\aeid[i]\ \text{occurs in}\ \acontext[i].A$, and (ii)
  $\aeid[i]\ \text{occurs in}\ \acontext[i+1].\aqueue$, considering
  addition modulo $n$.
\end{definition}

We repeat the figure of~\autoref{sec:semantics} representing a
deadlock state . Notice that in the queues of each of these contexts
there is a request of an event that is currently holding the previous
context in the chain (shown with the incoming arrows marked
$req(e_i)$), therefore closing the cycle.

\begin{center}
  \includegraphics[scale=.25]{figures/ddlock-crop}
\end{center}

\begin{lemma}
  \label{lem:lock-lub}
  For each event $\aeid$, and a state $(\aeventset, \acontextset)$
  such that there exists a context $\acontext \in \acontextset$ with
  $\aeid \in \acontext.A$, whenever
  $\mathsf{dom}(\acontextset, \mathsf{target}(\aeid)) =
  \acontext[\ell]$
  we have that $\aeid \in \acontext[\ell].A$.
\end{lemma}
\noindent In words, whenever an event $\aeid$ is executing in any
context, it is also activated in the dominator context corresponding
to the events target context according to $\acontextset$.
\begin{proof}
  We notice first that the only rules that allow events to be added to
  the activation of a context are the rules
  of~\autoref{fig:activation}.%  with the exception of \textsc{Event
    % Commit}. 
  
  Moreover, notice that for each of these rules, an item already
  existed in the queue of the context with the necessary event
  id. These are the premisses of the form
  $\acontext[0].\aqueue = (\aeid, \_, \dots)$. It is therefore
  sufficient to show that whenever a request is added to a queue, then
  either (i) it effectively is the dominator context, or (ii), the parent
  context contains $\aeid$ in its activations before enqueuing the
  request. Finally we have to show that no event is removed from an
  activation prematurely, but this is trivial, since the only rule
   which removes events from the activations is \textsc{Event
    Return \& Commit}, which removes all the $\aeid$ atomically from
  all contexts as shown in~\autoref{lem:lock-lub}.

  Conditions (i) and (ii) above are easy to check by inspection on the
  rules that can add requests in the queues of a context. For (i) we have
  that newly arrived events are always added with a request
  $(\aeid, \_, \_, \mathsf{lub}\ (\mathsf{event}\ \acontext[i]), \_)$ in
  the LUB context if it is not directly the target. For (ii) we can
  check the rules that that add elements to the queues (\textsc{Synch
  Call}, \textsc{ASynch Call}) require the parent context to have the
  event $\aeid$ in their activations.
\end{proof}

\begin{corollary}
  \label{cor:path-lock}
  For any reachable configuration $\aconf$, context
  $\acontext[0] \in \acontextset$, and event $\aeid \in \aeventset$
  such that $\aeid \in \acontext[0].A$ we have that
  $\aeid \in
  \mathsf{dom}(\mathsf{target}(\aeid),\acontextset).A$,
  and there exists a path of contexts
  $\mathsf{target}(\aeid) \ \cdot\ \acontext[1] \ \cdot\ \dots \
  \cdot\ \acontext[n] \ \cdot\ \acontext[0]$
  in $\acontextset$ -- considered as a graph -- from
  $\mathsf{target}(\aeid)$ to $\acontext[0]$ such that for each
  $i \in [1,n]$ we have $\aeid \in \acontext[i].A$.
\end{corollary}
\begin{proof}
  This is a direct consequence of (i)~\autoref{lem:lock-lub}, the fact
  that $\acontextset$ is a directed-acyclic graph, and (iii)
  the fact that events are only ever deactivated (i.e. removed from
  contexts activation sets) by the rule \textsc{Event Return \&
    Commit} which removes the event once and for all form the whole
  context set $\acontextset$.
\end{proof}

The following lemma states that elements involved in a deadlock cycle
must share a common dominator. This is the critical observation to
avoid deadlocks. 
\begin{lemma}
  \label{lem:unique-lub}
  Let us consider a deadlock state $(\aeventset, \acontextset)$, such
  that $\acontextset{}$ is a directed-acyclic-graph (DAG) as
  prescribed by the \aeoncore{} discipline. Moreover, let us assume
  that if an event $\aeid$ is either enqueued in a context
  $\acontext[]$ (i.e. $\aeid \in \acontext[].\aqueue$), or it is
  currently activated in it (i.e.
  $\aeid \in \activated{\acontext[]}$), then either $\acontext[]$ is
  the dominator of $\aeid$'s target
  ($\acontext[] = \mathsf{dom}(\mathsf{target}(\aeid),
  \acontextset)$),
  or a parent of $\acontext[]$ contains the event $\aeid$ in its
  activations.  Then, we have that all the contexts involved in the
  deadlock (as per~\autoref{def:deadlock}) have a unique dominator in
  $\acontextset$. Formally, $\mathsf{lub}(\acontextset, \{\acontext[]\
  |\ \acontext \in \text{deadlock of}\
  \acontextset\}) \in \mathsf{desc}(\mathsf{dom}(\mathsf{target}(\aeid),\acontextset))$.
\end{lemma}
\begin{proof}
  We proceed by induction on the number of contexts involved in the
  deadlock of state $(\aeventset, \acontextset)$. In particular, we
  relax the condition of there being a cycle, to requiring only that
  there is a path in between any two contexts (as opposed to a
  cycle). 
  We consider that there is a bidirectional edge between $\acontext[0]
  \in \acontextset$ and $\acontext[1] \in \acontextset$ if there
  exists an event $\aeid \in \aeventset$ such that $\aeid \in
  \activated{\acontext[0]}$ and $\aeid \in \acontext[1].\aqueue$, or
  viceversa. Then, we are interested in the length of the path formed
  with these bi-directional edges. 
  
  In the basic case, with only two contexts $\acontext[0]$ and
  $\acontext[1]$, we have that since in at least one of the two
  contexts one event is activated, and the other is enqueued, then
  both contexts share a common ancestor, which is guaranteed
  by~\autoref{cor:path-lock}. This concludes the case by considering
  the dominator of this common ancestor in $\acontextset$.

  In the inductive case we know there is a unique context that is the
  dominator of $\acontext[0]$, ..., $\acontext[n]$ in
  $\acontextset$. We also know that at least one of these contexts has
  an event activated which is in the queue an additional context
  $\acontext[n+1]$ or viceversa. Then, there are two cases: either (i)
  $\mathsf{dom}(\acontext[0], ..., \acontext[n], \acontext[n+1])
  = \mathsf{dom}(\acontext[0], ..., \acontext[n])$
  and we conclude the case, or (ii) otherwise, by the definition of
  \textsf{share} in~\autoref{sec:pmodel}, we have that
  the
  $\acontext[n+1] \in \mathsf{desc}(\mathsf{dom}(\acontext[0], ...,
  \acontext[n]))$.
  Therefore, by the definition of $\mathsf{share}$, also
  in~\autoref{sec:pmodel}, the dominator of the context
  containing the event that issued the call in $\acontext[n+1]$ has to
  also dominate $\mathsf{dom}(\acontext[0], ..., \acontext[n])$, which
  concludes the case.
\end{proof}

We can now state the deadlock freedom theorem of~\autoref{sec:semantics}.
\begin{theorem}
  The semantics of \aeoncore{} guarantees that no deadlock state can
  be reached. 
\end{theorem}
\begin{proof}
  We consider a proof by contradiction. Let us assume that there is a
  first state $(\aeventset, \acontextset)$ in a run of the semantics
  of~\autoref{fig:global-step} containing a deadlock as
  per~\autoref{def:deadlock}. Then, combining~\autoref{lem:unique-lub}
  and~\autoref{lem:lock-lub} we obtain a contradiction, since both
  events (one of which requires exclusive access) must be activated in
  the common dominator. 
\end{proof}

% \gp{I'm ignoring the $\readonly$ case. It's easy to add, but I have to
% do it. }

\paragraph{Linearizability.}~In this case we prove that the semantics of \aeoncore{} is
linearizable. Let us start by stating some simple properties of the
semantics. 

\begin{lemma}[Exclusive Access]
  \label{lem:exclusive}
  Given a trace
  $\vec{\omega} = (\aeventset_0, \acontextset_0) \xrightarrow{}
  (\aeventset_0, \acontextset_0) \dots \xrightarrow{} (\aeventset_n,
  \acontextset_n)$,
  assume that two events $\aeid[0]$ and $\aeid[1]$ access at least one
  coinciding context, say $\acontext$, in $\vec{\omega}$. We have that for any
  configuration $\aconf$ appearing in $\vec{\omega}$:
  \begin{compactenum}[1]
  \item
    $\mathsf{dom}(\acontextset,\mathsf{target}(\aeid[0])) \in
    \mathsf{desc}(\mathsf{dom}(\acontextset,\mathsf{target}(\aeid[1])))$,
    or\\
    $\mathsf{dom}(\acontextset,\mathsf{target}(\aeid[1])) \in
    \mathsf{desc}(\mathsf{dom}(\acontextset,\mathsf{target}(\aeid[0])))$,
    and
  \item $\aeid[0] \notin \activated{\acontext}$ or
    $\aeid[1] \notin \activated{\acontext}$.
  \end{compactenum}
\end{lemma}
\begin{proof}
  The claim 1 is a direct consequence of $\acontextset$ forming a DAG,
  ~\autoref{cor:path-lock}, ~\autoref{lem:lock-lub}, and the fact that
  both events operate on a common context $\acontext$. The claim 2 is
  a direct consequence of claim 1 in combination
  with~\autoref{cor:path-lock} and ~\autoref{lem:lock-lub}. 
\end{proof}

\begin{figure}[!t]
  \centering
    \begin{tikzpicture}
      \matrix (m) [matrix of math nodes,row sep=3em,column
      sep=2em,minimum width=2em] {
        & (\aeventset, \acontextset_0) \\
        (\aeventset,\acontextset') &  & (\aeventset, \acontextset'') \\
        & (\aeventset, \acontextset_1)\\};
      \path[-stealth] 
      (m-1-2) edge [dashed] node [left] {$\acontext[1]$} node [right] {$e_1$} (m-2-3) 
      (m-2-3) edge [dashed] node [left] {$\acontext[0]$} node [right] {$e_0$} (m-3-2) 
      (m-1-2) edge node [right] {$\acontext[0]$} node [left] {$e_0$} (m-2-1)
      (m-2-1) edge node [right] {$\acontext[1]$} node [left] {$e_1$} (m-3-2);
    \end{tikzpicture}  
  \caption{Commutativity of independent events}
  \label{fig:commutativity1}
\end{figure}

The following lemma was presented in~\autoref{sec:semantics}. Here we
restate it and provide it's proof. Similarly, we
repeat~\autoref{fig:commutativity1} to ease of presentation. 

\begin{lemma}[Commutativity]
  \label{lem:commuatativity}
  Consider two consecutive transitions where we assume two
  contexts $\acontext[0], \acontext[1] \in \acontextset$, and two
  events $e_0, e_1 \in \aeventset$:
  \[(\aeventset, \acontextset_0)
  \underset{e_{0}}{\xrightarrow{\acontext[0]}} (\aeventset,
  \acontextset') \underset{e_{1}}{\xrightarrow{\acontext[1]}}
  (\aeventset, \acontextset_1)\]
  Here we denote with the arrow
  $\underset{e}{\xrightarrow{\acontext[]}}$ the fact that the
  transition involved the event identifier $e$ and it was performed in
  the context $\acontext[]$.%\footnote{Not to be confused with the
    %labels of Figures~\ref{fig:small-step}-\ref{fig:activation}.} 
  We have that if either $\acontext[0] \neq \acontext[1]$ or
  $e_0.\aaccess = e_1.\aaccess = \readonly$, there exists an
  intermediary context set $\acontextset''$ such that the following
  transitions are also valid:
  \[(\aeventset, \acontextset_0) \underset{e_{1}}{\xrightarrow{\acontext[1]}}
  (\aeventset, \acontextset'') \underset{e_{0}}{\xrightarrow{\acontext[0]}}
  (\aeventset, \acontextset_1)\]
  \autoref{fig:commutativity1} depicts this lemma, where dashed arrows
  represent the existential transitions required by the lemma. 
  % \label{lem:commutativity}
\end{lemma}
\begin{proof}
  % Firstly, observe that if any of $e_0.\aaccess$ or $e_1.\aaccess$ is
  % $\exclusive$, then the two consecutive transitions are not possible
  % by~\autoref{lem:exclusive}. 
  The case where the two events are $\readonly$ is
  trivial. By~\autoref{lem:exclusive} we have that if any of the
  events is $\exclusive$, then $\acontext[0] \neq
  \acontext[1]$.
  Moreover, we have that
  $\activated{\mathsf{LUB}(\acontextset),\acontext[0]} = \{e_0\}$ and
  $\activated{\mathsf{LUB}(\acontextset,\acontext[1])} = \{e_1\}$.
  Hence, by the definition of $\mathsf{LUB}$ we have that
  $\mathsf{desc}(\acontext[0]) \cap \mathsf{desc}(\acontext[1]) =
  \emptyset$.
  It is not hard to see then, that the two events operate on disjoint
  portions of the graph, and therefore the transitions commute
  immediately.
\end{proof}

\begin{corollary}
  \label{cor:push-forward}
  Consider a sequence of transitions, where we use $\bar{\aeid}$
  denotes any of the events in, 
  \[\alpha\ =\ (\aeventset, \acontextset_0) \xrightarrow[\bar{e_0}]{} 
  (\aeventset, \acontextset_1,) \xrightarrow[\bar{e_1}]{}\ \dots\ \xrightarrow[\bar{e_{n-1}}]{} 
  (\aeventset,\acontextset_n)\]
  where no step except the last one is a commit event. We can conclude
  that there exists an equivalent trace 
  \[\alpha' = (\aeventset, \acontextset_0) \xrightarrow[\delta(\bar{e_{0}})]{}
  (\aeventset, \acontextset'_1) \xrightarrow[\delta(\bar{e_{1}})]{}\ \dots\ \xrightarrow[\delta(\bar{e_{n-1}})]{} 
  (\aeventset, \acontextset_n)\]
  where $\delta$ is an bijection from $\{\bar{e_0}, \dots, \bar{e_{n-1}}\}$ to
  itself, such that there exists an $m \in [0,n-1]$ with
  (i) for all $i<m$ we have $\delta(\bar{e_i}) = \bar{e_{m-1}}$, and (ii) for each $i
  \geq m$, $\delta(\bar{e_{i}}) \neq \bar{e_{n-1}}$. Essentially, the bijection
  $\delta$ pushes all transitions of $\bar{e_{n-1}}$ to the front. 
\end{corollary}
\noindent Notice that the initial and final configurations are the same.
\proof{This is a trivial consequence of the lemma above, considering
  that all transitions that need to be reordered correspond to
  different (concurrent) events.}

As we did in~\autoref{sec:meta-properties}, we consider an alternative
semantics of \aeoncore{} which allows at most one event at a time
(see~\autoref{sec:meta-properties}). As before, we call this the
\emph{linear semantics of \aeon{}} and denote it with the special
arrow ``$\twoheadrightarrow$'' and denote context sets generated by
this semantics as $\hat{\acontextset}$.

The proof of linearizability shows that the \emph{linear semantics of
  \aeoncore{}} can simulate the semantics of \aeoncore{}. To that end
we consider as simulation relation between configurations of the two
different semantics. We denote by $\mathcal{A}ct(\acontextset)$ the set
of events that are activated in any context of $\acontextset$. 

We consider as simulation relation between configurations of the two
different semantics. 

\begin{definition}[Simulation Relation]
  We define the following simulation relation between a configuration
  of the linear semantics of \aeon{},
  $(\aeventset, \hat{\acontextset})$, with a configuration of the
  low-level configurations of \aeon{}, $(\aeventset, \acontextset)$,
  denoted by
  \[(\aeventset, \hat{\acontextset})\ \mathcal{R}\ (\aeventset, \acontextset)\] 
  iff the following conditions are met:
  \begin{compactitem}
  \item[(i)] $\mathcal{A}ct(\hat{\acontextset}) = \emptyset$, and
  \item[(ii)] $(\aeventset, \hat{\acontextset}) \xrightarrow{*} (\aeventset, \acontextset')$
  \end{compactitem}
\end{definition}

We then prove that the semantics of linear \aeon{} simulates the
semantics of low-level \aeon{} by showing that the diagram below
commutes. This amounts to proving that each time we start with a pair
of similar configurations, whenever the low-level semantics makes a
step, there exists a step in the high-level semantics that can
simulate exactly the same behavior. Notice in particular, that the
event sets $\aeventset$ in any two similar configurations are
identical, meaning that transitions that modify the event set must be
matched one to one.

\begin{figure}[!h]
  \centering
    \begin{tikzpicture}
      \matrix (m) [matrix of math nodes,row sep=3em,column
      sep=4em,minimum width=2em] {
        (\aeventset, \hat{\acontextset}) & (\aeventset', \hat{\acontextset}') \\
        (\aeventset, \acontextset) & (\aeventset', \acontextset') \\};
      \path[-stealth] (m-1-1) edge [-] node [left] {$\mathcal{R}$}
      (m-2-1) edge [dashed] node [above] {*} (m-1-2)
      (m-2-1.east|-m-2-2) edge (m-2-2) (m-1-2) edge [dashed,-] node
      [right] {$\mathcal{R}$} (m-2-2);
    \end{tikzpicture}  
  \caption{\aeon{} simulation diagram}
  \label{fig:simulation}
\end{figure}

\begin{theorem}[Simulation]
  The relation $\mathcal{R}$ defined above is a weak-simulation from
  the low-level semantics of \aeon{} to the linear semantics of
  \aeon{}, as shown in~\autoref{fig:simulation}.
\end{theorem}
\begin{proof}
  We assume a pair of configurations related by the relation
  $\mathcal{R}$. Let them be $(\hat{\aeventset, \acontextset})\
  \mathcal{R}\ (\aeventset, \acontextset)$.

  The proof proceeds by case analysis on the transition taken by the
  configuration $(\aeventset, \acontextset)$ of standard $\aeon{}$.
  Importantly, we \emph{only need to cater for transitions that modify
    the event set} $\aeventset$, since all other transitions
  immediately preserve the relation $\mathcal{R}$, as the second
  condition of the definition of the relation requires that the
  configuration $(\aeventset, \hat{\acontextset})$ can reach
  $( \aeventset, \acontextset)$, and evidently, similar steps can be
  taken to preserve the relation. Hence, we consider only transitions
  that modify the event sets. These are: \textsc{Event Call UnShared},
  \textsc{Event Call Shared} and \textsc{Event Return}.
  \begin{compactitem}
  \item \textsc{Event Call UnShared} and \textsc{Event Call
      Shared}. The transitions taken by these rules are trivially
    matched by the linear semantics, since these events are only added
    to the tail of the queue (in both configurations). % \gp{Not sure if
    % I need to say more here.}
  \item \textsc{Event Return}. This is the only important step, since
    it is here that the linear semantics (i.e. the configuration
    $(\aeventset, \hat{\acontextset})$) must make actual transitions.
    In this case, we can directly apply~\autoref{cor:push-forward} to
    obtain the conclusion, since we have from~\ref{lem:lock-no-unlock}
    and~\ref{rem:return-commit} that the committing event was the only
    one to touche these contexts (i.e. all other concurrent events are
    disjoint), and the event continued to hold these contexts until
    this commit step. 
    % \gp{Not sure if this is too obvious, or if I need to add something
    % here. }
  \end{compactitem}
\end{proof}

Evidently, \emph{the simulation above induces a linearizability proof},
where events are linearized at their commit point. 

\begin{corollary}[Linearizability]
  Since the linear \emph{semantics of \aeoncore{}} is linear, and
  it does not reorder non-overlapping events, \autoref{thm:sim}
  implies that the semantics of \aeoncore{} enforces linearizability
  of events. 
\end{corollary}

\paragraph{Parallelism}

\begin{definition}[Independent Events]
  Given a trace $\vec{\omega}$ and events $e_0, e_1 \in \aeventset$,
  we say that $e_0$ and $e_1$ are independent in $\vec{\omega}$ iff
  whenever $\vec{\omega}$ can be decomposed as
  \[\vec{\omega} = \vec{\omega_0} \cdot (\aeventset, \acontextset_0)
  \underset{e_{0}}{\xrightarrow{\acontext[0]}} (\aeventset,
  \acontextset_1) \cdot \vec{\omega_1} \cdot (\aeventset,
  \acontextset_2)\underset{e_{1}}{\xrightarrow{\acontext[1]}}
  (\aeventset, \acontextset_3) \cdot \vec{\omega_{3}}\] 
  we have that $\acontext[0] \neq \acontext[1]$.
\end{definition}

\begin{theorem}\label{th:indevents}[Independence $\Rightarrow$ Parallelism]
  Consider a trace $\vec{\omega}$ and two independent events
  $e_0, e_1 \in \aeventset$. We have that whenever 
  \[\vec{\omega} = \vec{\omega_0} \cdot (\aeventset, \acontextset_0)
  \underset{e_{0}}{\xrightarrow{\acontext[0]}} (\aeventset,
  \acontextset_1) \underset{e_{1}}{\xrightarrow{\acontext[1]}}
  (\aeventset, \acontextset_2) \cdot \vec{\omega_{3}}\] 
  there exists an equivalent trace 
  \[\vec{\omega} = \vec{\omega_0} \cdot (\aeventset, \acontextset_0)
  \underset{e_{1}}{\xrightarrow{\acontext[1]}} (\aeventset,
  \acontextset') \underset{e_{0}}{\xrightarrow{\acontext[0]}}
  (\aeventset, \acontextset_2) \cdot \vec{\omega_{3}}\] 
  where the order of the transitions of $e_0$ and $e_1$ is reversed. 
\end{theorem}
\begin{proof}This is an immediate consequence
  of~\autoref{lem:commuatativity}.
\end{proof} 
\noindent In a nutshell this theorem establish that the order of steps of events
$e_0$ and $e_1$ is inconsequential, and therefore they can be
evaluated in any order (i.e. in parallel). 

% \input{ownership-check}

%%% Local Variables:
%%% mode: latex
%%% TeX-master: "main"
%%% End:
